# Supplementary material for: The Hidden Pitfalls of the Cosine Similarity Loss
Source: arXiv:2406.16468 source file (2024-06-24)
Supplement: Supplementary file 1 [file eccv_9_appendix.tex]

\section{Proofs}
\subsection{Proof of Proposition~\ref{prop:cos_sim_grads}}
\label{prf:prop_grad_grows}
\begin{proof}
    We are taking the gradient of $\mathcal{L}^\mathcal{A}_i$ as a function of $z_i$. The principal idea is that the gradient has a term with direction $\hat{z}_j$ and a term with direction $-\hat{z}_i$. We then disassemble the vector with direction $\hat{z}_j$ into its component parallel to $z_i$ and its component orthogonal to $z_i$. In doing so, we find that the two terms with direction $z_i$ cancel, leaving only the one with direction orthogonal to $z_i$.
    
    Writing it out fully, we have $\mathcal{L}^\mathcal{A}_i = z_i^\top z_j / (||z_i|| \cdot ||z_j||)$. Taking the gradient of this then amounts to using the quotient rule, with $f = z_i^\top z_j$ and $g = ||z_i|| \cdot ||z_j|| = \sqrt{z_i^\top z_i} \cdot \sqrt{z_j^\top z_j}$. Taking the derivative of each, we have
    \begin{align*}
        f' &= \mathbf{z}_j \\
        g' &= ||z_j|| \frac{z_i}{\sqrt{z_i^\top z_i}} = ||z_j|| \frac{\mathbf{z}_i}{||z_i||} \\
        \implies \frac{f' g - g' f}{g^2} &= \frac{\left(\mathbf{z}_j \cdot ||z_i|| \cdot ||z_j|| \right) - \left(||z_j|| \frac{\mathbf{z}_i}{||z_i||} \cdot z_i^\top z_j \right)}{||z_i||^2 \cdot ||z_j||^2} \\
        &= \frac{\mathbf{z}_j}{||z_i|| \cdot ||z_j||} - \frac{\mathbf{z}_i z_i^\top z_j}{||z_i||^3 ||z_j||},
    \end{align*}
    where we use boldface $\mathbf{z}$ to emphasize which direction each term acts along. We now substitute $\cos(\phi_{ij}) = z_i^\top z_j / (||z_i|| \cdot ||z_j||)$ in the second term to get
    \begin{equation}
        \label{eq:quotient_rule}
        \frac{f' g - g' f}{g^2} = \frac{\hat{z}_j}{||z_i||} - \frac{\mathbf{z}_i \cos(\phi)}{||z_i||^2}
    \end{equation}

    It remains to separate the first term into its sine and cosine components and perform the resulting cancellations. To do this, we take the projection of $\hat{z}_j = \mathbf{z}_j / ||z_j||$ onto $\mathbf{z}_i$ and onto the plane orthogonal to $\mathbf{z}_i$. The projection of $\hat{z}_j$ onto $\mathbf{z}_i$ is given by
    \[ \cos \phi_{ij} \frac{\mathbf{z}_i}{||z_i||} \]
    while the projection of $\mathbf{z}_j / ||z_j||$ onto the plane orthogonal to $\mathbf{z}_i$ is
    \[ \left( \mathbf{I} - \frac{z_i z_i^\top}{||z_i||^2} \right) \frac{\mathbf{z}_j}{||z_j||}. \]
    It is easy to assert that these components sum to $\mathbf{z}_j/||z_j||$ by replacing the $\cos \phi_{ij}$ by $\frac{z_i^\top z_j}{||z_i||\cdot ||z_j||}$.

    We plug these into Eq.~\ref{eq:quotient_rule} and cancel the first and third term to arrive at the desired value:
    \begin{align*}
        \frac{f' g - g' f}{g^2} = &\frac{1}{||z_i||} \cos \phi \frac{\mathbf{z}_i}{||z_i||} \\
        &+ \frac{1}{||z_i||} \cdot \left( \mathbf{I} - \frac{z_i z_i^\top}{||z_i||^2} \right) \frac{\mathbf{z}_j}{||z_j||} \\
        &- \frac{\mathbf{z}_i \cos(\phi)}{||z_i||^2} \\
        = &\frac{1}{||z_i||} \cdot \left( \mathbf{I} - \frac{z_i z_i^\top}{||z_i||^2} \right) \frac{\mathbf{z}_j}{||z_j||}.
    \end{align*}
\end{proof}

\subsection{Proof of Theorem~\ref{thm:convergence_rate}}
\label{prf:thm_convergence_rate}
We first restate the theorem:

Let $z_i$ and $z_j$ be positive embeddings with equal norm, i.e. $||z_i|| = ||z_j|| = \rho$. Let $z_i'$ and $z_j'$ be the embeddings after 1 step of gradient descent with learning rate $\gamma$. Then the change in cosine similarity is bounded from above by:
\begin{equation*}
    \hat{z}_i'^\top \hat{z}_j' - \hat{z}_i^\top \hat{z}_j < \frac{\gamma \sin^2 \phi_{ij}}{\rho^2} \left[ 2 - \frac{\gamma \cos \phi}{\rho^2} \right].
\end{equation*}

\noindent We now proceed to the proof:
\begin{proof}
    Let $z_i$ and $z_j$ be two embeddings with equal norm\footnote{We assume the Euclidean distance for all calculations.}, i.e. $||z_i|| = ||z_j|| = \rho$. We then perform a step of gradient descent to maximize $\hat{z}_i^\top \hat{z}_j$. That is, using the gradients in \ref{prop:cos_sim_grads} and learning rate $\gamma$, we obtain new embeddings $z_i' = z_i + \frac{\gamma}{||z_i||} (\hat{z}_j)_{\perp z_i}$ and $z_j' = z_j + \frac{\gamma}{||z_j||} (\hat{z}_i)_{\perp z_j}$. Going forward, we write $\delta_{ij} = (\hat{z}_j)_{\perp z_i}$ and $\delta_{ji} = (\hat{z}_i)_{\perp z_j}$, so $z_i' = z_i + \frac{\gamma}{\rho} \delta_{ij}$ and $z_j' = z_j + \frac{\gamma}{\rho} \delta_{ji}$. Notice that since $z_i$ and $\delta_{ij}$ are orthogonal, by the Pythagorean theorem we have $||z_i'||^2 = ||z_i||^2 + \frac{\gamma^2}{\rho^2}||\delta_{ij}||^2 \geq ||z_i||^2$. Lastly, we define $\rho' = ||z_i'|| = ||z_j'||$.

    We are interested in analyzing $\hat{z}_i'^\top \hat{z}_j' - \hat{z}_i^\top \hat{z}_j$. To this end, we begin by re-framing $\hat{z}_i'^\top \hat{z}_j'$:
    \begin{align*}
        \hat{z}_i'^\top \hat{z}_j' &= \left(\frac{z_i + \frac{\gamma}{\rho} \delta_{ij}}{\rho'}\right)^\top \left(\frac{z_j + \frac{\gamma}{\rho} \delta_{ji}}{\rho'}\right) \\
        &= \frac{1}{\rho'^2}\left[ z_i^\top z_j + \gamma \frac{z_i^\top \delta_{ji}}{\rho'} + \gamma \frac{z_j^\top \delta_{ij}}{\rho'} + \gamma^2 \frac{\delta_{ij}^\top \delta_{ji}}{\rho'^2} \right].
    \end{align*}

    We now consider that, since $\delta_{ij}$ is the projection of $\hat{z}_j$ onto the subspace orthogonal to $z_i$, we have that the angle between $z_i$ and $\delta_{ji}$ is $\pi/2 - \phi_{ij}$. Plugging this in and simplifying, we obtain
    \begin{align*}
        z_i^\top \delta_{ji} &= ||z_i|| \cdot ||\delta_{ji}|| \cos (\pi/2 - \phi_{ij}) \\
        &= ||z_i|| \cdot ||\delta_{ji}|| \sin \phi_{ij} \\
        &= \rho \sin^2 \phi_{ij}.
    \end{align*}
    By symmetry, the same must hold for $z_j^\top \delta_{ij}$.
    
    Similarly, we notice that the angle $\psi_{ij}$ between $\delta_{ij}$ and $\delta_{ji}$ is $\psi_{ij} = \pi - \phi_{ij}$. The reason for this is that we must have a quadrilateral whose four internal angles must sum to $2\pi$, i.e. $\psi_{ij} + \phi_{ij} + 2 \frac{\pi}{2} = 2 \pi$. Thus, we obtain $\delta_{ij}^\top \delta_{ji} = ||\delta_{ij}|| \cdot ||\delta_{ji}|| \cos(\psi) = -\sin^2 \phi_{ij} \cos \phi_{ij}$.

    We plug these back into our equation for $\hat{z}_i'^\top \hat{z}_j'$ and simplify:
    \begin{align*}
        \hat{z}_i'^\top \hat{z}_j' &= \frac{1}{\rho'^2}\left[ z_i^\top z_j + \gamma \frac{z_i^\top \delta_{ji}}{\rho} + \gamma \frac{z_j^\top \delta_{ij}}{\rho} + \gamma^2 \frac{\delta_{ij}^\top \delta_{ji}}{\rho^2} \right] \\
        &= \frac{1}{\rho'^2}\left[ z_i^\top z_j + \gamma \frac{\rho \sin^2 \phi_{ij}}{\rho} + \gamma \frac{\rho \sin^2 \phi_{ij}}{\rho} - \gamma^2 \frac{\sin^2 \phi_{ij} \cos \phi_{ij}}{\rho^2} \right] \\
        &= \frac{1}{\rho'^2}\left[ z_i^\top z_j + 2 \gamma \sin^2 \phi_{ij} - \gamma^2 \frac{\sin^2 \phi_{ij} \cos \phi_{ij}}{\rho^2} \right].
    \end{align*}

    We now consider the original term in question:
    \begin{align*}
        \hat{z}_i'^\top \hat{z}_j' - \hat{z}_i^\top \hat{z}_j &= \frac{1}{\rho'^2}\left[ z_i^\top z_j + 2 \gamma \sin^2 \phi_{ij} - \gamma^2 \frac{\sin^2 \phi_{ij} \cos \phi_{ij}}{\rho^2} \right] - \frac{z_i^\top z_j}{\rho^2} \\
        &\leq \frac{1}{\rho^2}\left[ z_i^\top z_j + 2 \gamma \sin^2 \phi_{ij} - \gamma^2 \frac{\sin^2 \phi_{ij} \cos \phi_{ij}}{\rho^2} \right] - \frac{z_i^\top z_j}{\rho^2} \\
        &= \frac{1}{\rho^2}\left[ 2 \gamma \sin^2 \phi_{ij} - \gamma^2 \frac{\sin^2 \phi_{ij} \cos \phi_{ij}}{\rho^2} \right] \\
        &= \frac{\gamma \sin^2 \phi_{ij}}{\rho^2}\left[ 2 - \frac{\gamma \cos \phi_{ij}}{\rho^2} \right]
        &\leq \frac{2 \gamma \sin^2 \phi_{ij}}{\rho^2}
    \end{align*}
    
    This concludes the proof.
\end{proof}

\subsection{Proof of Corollary~\ref{cor:grad_grows}}
\label{prf:cor_grad_grows}
\begin{proof}
    We are interested in the gradient of $\mathcal{L}_i^\mathcal{R}$ with respect to $z_i$. By the chain rule, we get
    \begin{align*}
        \nabla_i^\mathcal{R} &= \frac{\sum_{k \not\sim i} \text{sim}(z_i, z_k) \frac{\partial \frac{z_i^\top z_k}{||z_i|| \cdot ||z_k||}}{\partial z_i}}{\sum_{k \not\sim i} \text{sim}(z_i, z_k)} \\
        &= \frac{\sum_{k \not\sim i} \text{sim}(z_i, z_k) \frac{\partial \frac{z_i^\top z_k}{||z_i|| \cdot ||z_k||}}{\partial z_i}}{S_i}
    \end{align*}
    It remains to substitute the result of Prop. \ref{prop:cos_sim_grads} for $\partial \frac{z_i^\top z_k}{||z_i|| \cdot ||z_k||} / \partial z_i$.

    We sum this this with the gradients of the attractive term to obtain the full InfoNCE gradient, completing the proof.
\end{proof}

\subsection{Proof of Proposition~\ref{prop:unlikely_opp_halves}}
\label{prf:prop_opp_halves}

By \cite{distribution_of_cosine_sim}, the cosine similarity between two i.i.d. random variables drawn from $\mathcal{N}(0, \mathbf{I})$ has expected value $\mu = 0$ and variance $\sigma^2 = 1/d$, where $d$ is the dimensionality of the space. We therefore plug these into Chebyshev's inequality:
\begin{align*}
    &\text{Pr} \left[ \abs*{\frac{x_i^\top x_j}{||x_i||\cdot ||x_j||} - \mu} \geq k \sigma \right] \leq \frac{1}{k^2} \\
    \rightarrow & \text{Pr} \left[ \abs*{\frac{x_i^\top x_j}{||x_i||\cdot ||x_j||}} \geq \frac{k}{\sqrt{d}} \right] \leq \frac{1}{k^2}
\end{align*}

\noindent We now choose $k = \sqrt{d}(1 - \varepsilon)$, giving us
\[ \mathbb{P}\left[ \abs*{\frac{x_i^\top x_j}{||x_i|| \cdot ||x_j||}} \geq 1 - \varepsilon \right] \leq \frac{1}{d(1-\varepsilon)^2}.\]

It remains to remove the absolute values around the cosine similarity. Since the cosine similarity is symmetric around $0$, the likelihood that its absolute value exceeds $1 - \varepsilon$ is twice the likelihood that its value exceeds $1- \varepsilon$, concluding the proof.

We note that this is actually an extremely optimistic bound since we have not taken into account the fact that the maximum of the cosine similarity is 1.

\section{Experimental Setup}
\label{sec:experiment_setup}

Our default experimental pipeline uses a Resnet-18 backbone~\cite{resnet} and the default input-image augmentations as described in the SimCLR paper ~\cite{simclr}. We use the 3-layer projector described in \cite{simsiam} in each method's encoder. We default the projector's output dimensionality to 128 and 2048 for SimCLR and SimSiam/BYOL, respectively. SimCLR's projector does not use batch-norm while BYOL and SimSiam have it on all three layers (including the output). As mentioned in \cite{simsiam}, we use a two-layer predictor where the middle has dimensionality $512$ (to act as a simple autoencoder). The middle layer of the predictor has batch-norm while the last one does not. We begin our experiments with weight decay 1e-6 for SimCLR and 5e-4 in BYOL and SimSiam. Our learning rates are $0.6$ and $0.2$ for Simclr and SimSiam/BYOL and we use a cosine learning rate schedule with linear startup as described in \cite{simclr} with standard SGD and momentum 0.9. Unless stated otherwise, all of our experiments are done on the Cifar-10 dataset~\cite{cifar10} with batch size $b=512$. Due to compute restrictions, we use batch-size $128$ when running a Resnet-50 backbone and batch-size $512$ when running a Resnet-18 backbone. As mentioned, this leads to suboptimal performance on SimCLR, which requires large batch sizes. We also use the CIFAR100 datasets~\cite{cifar10} along with Imagenet-100~\cite{imagenet}. The 100 classes chosen for ImageNet-100 are in accordance with those used in~\cite{understanding_contr_learn} (specifically found \textcolor{blue}{\hyperref[https://github.com/ssnl/moco_align_uniform/blob/7ff7bfb1df1473936c8da880028d31dac40afbaf/scripts/imagenet100_classes.txt]{here}}). The anonymized code to recreate the SimCLR/SimSiam/BYOL experiments can be found at https://anonymous.4open.science/r/contrastive\_learning\_analysis-FC2C/. Experiments can be run using the file \texttt{CLA/experiments/default\_training.py}.

We use the Solo-Learn library \cite{solo-learn} to run Mocov2, Mocov3 and Dino. For Mocov2, we use a Resnet-50 backbone, we use the base $\tau =0.99$ and final $\tau: 0.999$ with learning rate $0.3$ and weight decay $1e-4$ with projection dimension $2048$ and queue size $4096$. For Mocov3, we use base $\tau=0.99$ and final $\tau=1$, with a learning rate of $3e-4$ and weight decay of $0.1$ with projection dimension as $4096$.
For Dino, we use $\tau=0.9995$ and final $\tau: 1.0$  with a learning rate $0.3$ and weight decay of $1e-6$ with projection dimension $2048$. 

\section{How One Might Fix the Opposite-Halves Effect}
\label{app:new_loss}

We use this space to finalize our study of the opposite-halves effect. We first recall the statement of this effect: when the angle $\phi_{ij}$ between embeddings $z_i$ and $z_j$ is close to $\pi$, the gradients of the cosine similarity go to 0. Since SSL models want positive pairs near one another in the latent space, this is clearly an undesired effect. Although we saw in Section~\ref{ssec:opp_halves_effect} that it does not occur in our studied datasets, it may be the case that it does occur in other settings.

The simplest method to overcome this would be to devise a new loss function that is similar to the cosine similarity but does not have the opposite-halves property. Formally, we want a loss function $\mathcal{L}'(\phi_{ij})$ such that:
\begin{enumerate}
    \item $\mathcal{L}'$ maximally recreates the cosine similarity when $0 \leq \phi_{ij} \leq \frac{\pi}{2}$, and
    \item $\mathcal{L}'$'s gradient norm continues to increase monotonically\footnote{We refer to the MSE loss function as an example of why monotonic increase is desirable.} over the domain $[\frac{\pi}{2}, \pi]$.
\end{enumerate}

To devise this loss function, consider the embedding\footnote{This is achieved in practice by \texttt{z\_j\_prime = ((z\_i + z\_j)/2).detach()}. We also add $\varepsilon \rightarrow 0$ to it so that $z_j' \neq 0$.} $z_j' = \frac{z_i + z_j}{2}$. Then, the cosine similarity between $z_i$ and $z_j'$ has a norm proportional to $\sin \frac{\phi_{ij}}{2}$ and is maximized when $z_i$ and $z_j$ are opposite one another on the hypersphere. We therefore define the \emph{strong cosine similarity} loss as
\begin{equation}
    \label{eq:strong_cos_sim}
    \mathcal{L}_i' = 2 \hat{z}_i^\top \hat{z}_j'.
\end{equation}

\noindent \begin{minipage}{0.55\textwidth}
We quickly verify that this is the natural choice for satisfying our two requirements. Assuming that $z_j'$ is not a function of $z_i$ and that $||z_i||=1$, the gradient of the strong cosine similarity loss has magnitude $||\nabla'|| = 2\sin \frac{\phi_{ij}}{2}$. We compare this to the gradient of the cosine similarity ($||\nabla|| = \sin \phi_{ij}$) in Figure \ref{fig:cos_grads} to the right. Specifically, we see that the two loss functions line up perfectly for $0 \leq \phi_{ij} \leq \pi / 4$, implying that nearby points experience similar attraction. However, whereas the cosine similarity gradient is $0$ at $\phi_{ij} = \pi$, the strong cosine similarity's gradient is maximized. Thus, according to the theory established in Section~\ref{ssec:theory_rel_work}, if the opposite-halves effect occurred, the strong cosine similarity should lead to a clear improvement over the standard one when training SSL models.
\end{minipage}
\quad \quad
\begin{minipage}{0.35\textwidth}
    %\vspace*{-1cm}
    \centering
    \includegraphics[width=\linewidth]{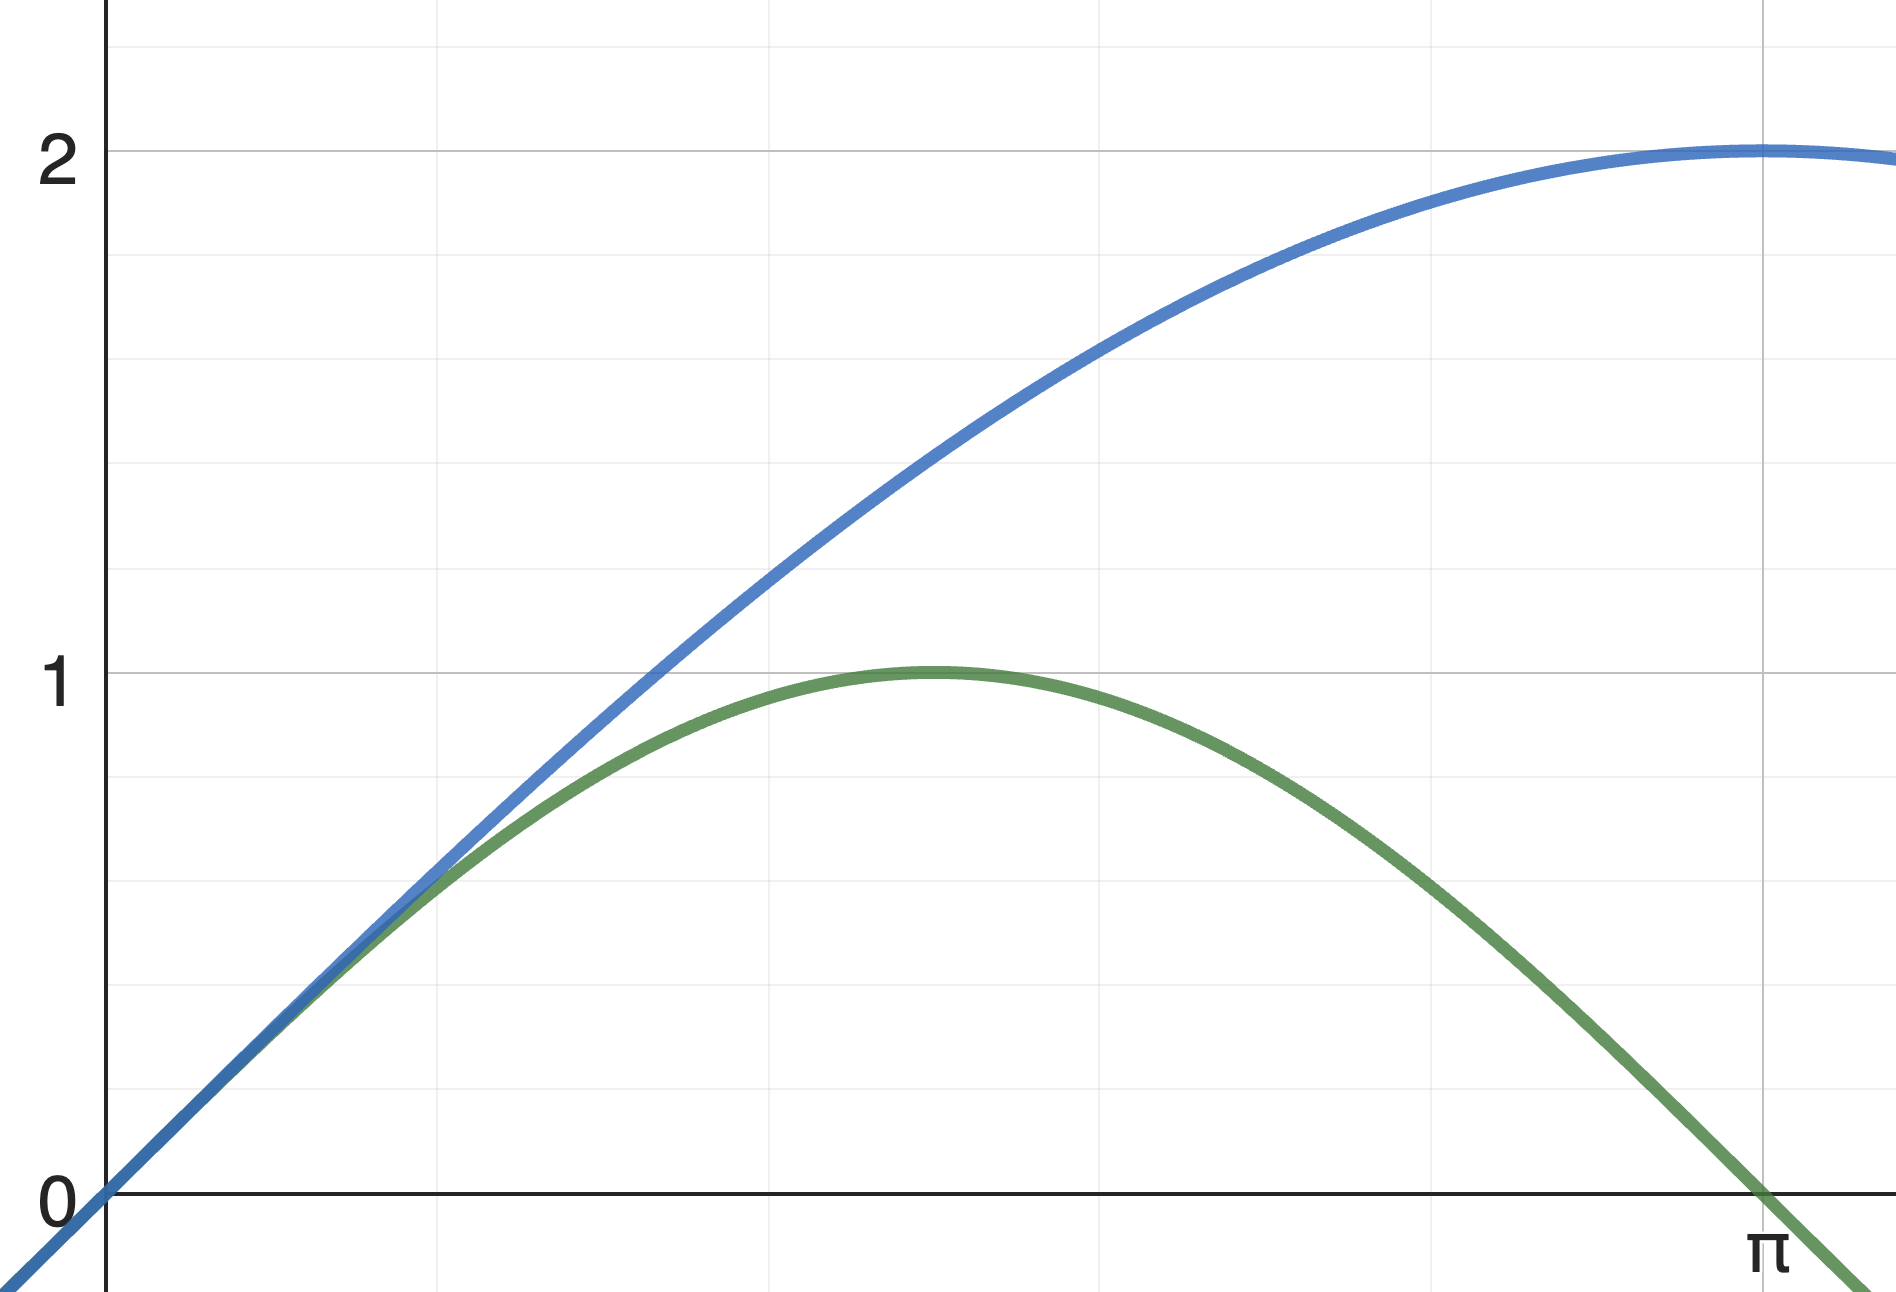}
    \captionof{figure}{A comparison of the cos. sim. gradient norm (green) and the \emph{strong} cos. sim. gradient norm (blue) as a function of $\phi_{ij}$.}
    \label{fig:cos_grads}
\end{minipage}
